# Supplementary material for: Stochastic Epidemic Models inference and diagnosis with Poisson Random Measure Data Augmentation
Source: arXiv:2004.10264 ancillary file (2020-04-21)
Supplement: Supplementary file 1 [file supplementary.pdf]

# Stochastic Epidemic Models inference and diagnosis with Poisson Random Measure Data Augmentation Appendix

Benjamin Nguyen-Van-Yen[a,b,*], Pierre Del Moral[c], Bernard Cazelles[b,d,e]

[a] *Institut Pasteur, Unité de Génétique Fonctionnelle des Maladies Infectieuses, UMR 2000 CNRS, Paris, France*

[b] *Institut de Biologie de l'ENS (IBENS), Ecole Normale Supérieure, CNRS, INSERM, Université PSL, 75005 Paris, France*

[c] *INRIA, Bordeaux Research Center, France*

[d] *International Center for Mathematical and Computational Modeling of Complex Systems (UMMISCO), UMI 209, UPMC/IRD, France*

[e] *iGLOBE, UMI CNRS 3157, University of Arizona, Tucson, Arizona, United States of America*

## A. Mathematical definitions

A discrete measure on the measurable space $(E, \mathcal{A})$ is a measure $\nu$ that puts mass on an at most countable subset of $E$,

$$\exists\ (x_n)_n \in E^{\mathbb{N}}, \nu(E \setminus \{x_n, n \in \mathbb{N}\}) = 0$$

It can be written as a linear combination of dirac measures on $E$.

$$\exists\ (a_n)_n \in {\mathbb{R}_+}^{\mathbb{N}}, \exists (x_n)_n \in E^{\mathbb{N}}, \nu = \sum_{i \geq 0} a_i \delta_{x_n}$$

Integration against a discrete measure reduces to summation

$$\int_E f\ d\nu = \sum_{i \in \mathbb{N}} a_i f(x_i)$$

Let $(\Omega, \mathcal{F}, (\mathcal{F}_t)_{t \geq 0}, \mathbb{P})$ be a filtered probability space.

Let $(E, \mathcal{B})$ be an euclidean space equipped with its canonical Borel $\sigma$-field,

Let $\lambda$ be a Lebesgue dominated measure.

A Poisson random measure (PRM) on $E$, with intensity measure $\lambda$ is a random counting measure such that the number of points in a measurable subset $A$ is Poisson distributed with parameter $\lambda(A)$. Additionally, the numbers of points in disjoint measurable subsets are independent. A succint presentation is given in [1].

*Corresponding author

A Markov pure jump process $X$ is a stochastic process $X : \Omega \times \mathbb{R}_+ \to E$, whose paths are càdlàg and constant in between jumps. An extensive presentation can be found in [2].

## B. Reformulation of a Markov jump process as a stochastic differential equation

Markov pure jump processes are characterized by events, which happen at exponential times with a certain rate, and which modify the system.

We will limit ourselves here to the simple case of processes taking values in $\mathbb{Z}^d$, but the results are more general and the reader can refer themselves to the literature, for example [3] or [4].

We consider a process taking values in $E = \mathbb{Z}^d$, with a finite number of events $K$. The $k$-th event happens with a rate $r_k : \mathbb{Z}^d \to \mathbb{R}_+$, and when it happens, the state changes from $x$ to $x + \mu_k$.

Let $(\nu_k)_{k\leq K}$ be independent standard PRMs, of intensity the Lebesgue measure on $\mathbb{R}_+ \times \mathbb{R}_+$.

Let $X_0$ be a random variable on $E$.

$$X_t = X_0 + \sum_{k\leq K} \int_0^t \int_{\mathbb{R}_+} \mathbb{1}_{u \leq r_k(X_{s^-})} \mu_k \nu_k(ds, du) \tag{B.1}$$

Solutions to the Poisson driven stochastic differential equation (B.1) are Markov pure jump processes, and their infinitesimal generator $L$ is such that for $\phi : E \to \mathbb{R}_+$ continuous, bounded and measurable,

$$L\ \phi(x) = \sum_{k\leq K} r_k(x) \left(\phi(x + \mu_k) - \phi(x)\right)$$

*Proof.* The problems of existence and uniqueness of the solution are not easy, and classically require the integrand to satisfy the linear growth and local Lipschitz conditions ([3], Theorem IV.9.1), which are not verified in our case, as the integrand is not continuous. The weaker conditions of [5] also do not hold.

Here we simply show that the equation does describe solutions that correspond to the typical continuous time Markov chain as simulated by Gillespie's algorithm.

Let us make the hypothesis that a solution $X$ exists and let us study its properties. The solution can only change value at atoms of the $(\nu_k)$, of which there are finitely many in a compact, almost surely. So the paths are constant by part. The solution is also continuous on the right almost surely, from the definition of Lebesgue integration. Thus the solution is a pure jump process.

We can show that $X$ is Markov by showing that the waiting time to the next jump is exponential. First, in the case with a single event $(r, \mu)$. Let us write $\nu = \sum_{n\in\mathbb{N}} \delta_{(t_n,u_n)}$. The next jump time after time $t$ is the time of the first atom of $\nu$, $(t_n, u_n)$, such that $u_n$ is below the rate $r(X_t)$.

$$s = \min\{t_n, n \in \mathbb{N}, t_n \geq t, u_n \leq r(X_t)\}$$

The process

$$s \mapsto N(s-t) = \nu\left([t,s] \times [0, r(X_t)]\right), s \geq t$$

is a homogeneous Poisson process of intensity $r(X_t)$. Thus the waiting time to the first event after $t$ is exponential, with rate $r(X_t)$, and the process has the Markov property. Similarly, with $K$ events, by superposition of independent Poisson random measures, the process

$$s \mapsto N(s-t) = \sum_{k \leq K} \nu_k\left([t,s] \times [0, r_k(X_t)]\right), s \geq t$$

is a homogeneous Poisson process of intensity $\sum_{k \leq K} r_k(X_t)$. Thus the waiting time to the first event after $t$ is exponential, with rate $\sum_{k \leq K} r_k(X_t)$, and the event $i$ happens with probability $\frac{r_i(X_t)}{\sum_{k \leq K} r_k(X_t)}$.

Let $C_b(E, \mathbb{R}_+)$ be the space of continuous bounded measurable functions from $E$ to $\mathbb{R}_+$. Let $(X_t^x)_t$ be a solution of (B.1) starting from $x$. We now determine the infinitesimal generator $L$ of the process, defined by

$$\forall \phi \in C_b(E, \mathbb{R}_+), \forall x \in E, L\ \phi(x) = \lim_{t \to 0^+} \frac{\mathbb{E}\left[\phi(X_t^x)\right] - \phi(x)}{t}$$

Let $\phi$ be a continuous bounded measurable function, and $x \in E$.

$$\begin{aligned}
&\mathbb{E}(\phi(X_t^x)) = \phi(x) + \sum_{k \leq K} \int_0^t \int_{\mathbb{R}_+} \mathbb{E}\left[\mathbb{1}_{u \leq r_k(X_{s^-}^x)} \left(\phi(X_{s^-}^x + \mu_k) - \phi(X_{s^-}^x)\right)\right]\ ds\ du \\
\iff &\mathbb{E}(\phi(X_t^x)) - \phi(x) = \sum_{k \leq K} \int_0^t \mathbb{E}\left[r_k(X_{s^-}^x)\left(\phi(X_{s^-}^x + \mu_k) - \phi(X_{s^-}^x)\right)\right]\ ds \\
\iff &\lim_{t \to 0^+} \frac{\mathbb{E}(\phi(X_t^x)) - \phi(x)}{t} = \sum_{k \leq K} \mathbb{E}\left[r_k(X_0^x)\left(\phi(X_0^x + \mu_k) - \phi(X_0^x)\right)\right] \\
\iff &L\ \phi(x) = \sum_{k \leq K} r_k(x)\left(\phi(x + \mu_k) - \phi(x)\right)
\end{aligned} \tag{B.2}$$

This corresponds to the usual notion of a continuous time Markov chain, with event $k$ happening at rate $r_k$ and changing the state by $\mu_k$. □

Additionnally, note that for the specific case of SIR type models, like the ones we have used as examples, there can be no explosion.

The only non-linear event that might cause problems is infection, which consumes susceptibles $S$. $S$ thus bounds the total number of infections that might happen, and $S < N$ the total population. The infection rate is proportional to $S$ and $I$, which are both bounded by $N$.

So the solution could explode only if the total population exploded. But the only events that change the total population are host births and host deaths, which happen respectively at a constant rate and at a linear rate. Therefore there can be no explosion.

## C. Reversibility of the MCMC proposal

MCMC relies on the ability to evaluate the posterior density. Discrete measures do not live in a Euclidean space, so we need to be explicit about what measure dominates the probability distribution for $\nu$.

We assume the parameters $\theta$ are indeed defined on a Euclidean space, and only concern ourselves with the problem of the posterior $\nu$ density. Let $\pi$ be the probability measure of a standard Poisson Random Measure, the prior density for $\nu$. By Bayes's theorem, $\mathbb{P}(\nu|D)$ is dominated by $\pi$, and thus it has a density with respect to $\pi$.

Then to define a valid proposal for $\nu$, we need to show that it is reversible with respect to $\pi$. Our proposal $Q_\nu$ consists in redrawing a given slice of time from the standard PRM process. The points in disjoint measurable sets of a PRM are independent, both their number and their position. As a consequence, the proposal $Q_\nu$ is reversible with respect to $\pi$, since it transforms a PRM sample into another (correlated) PRM sample.

For any two measures $\nu$ and $v$, and for any measurable set $C$, we define the measure $g_C(\nu, v)(A) = \nu(A \setminus C) + v(A \cap C)$ let $\nu(A, B, \mathcal{K}) = \sum_{k \in \mathcal{K}} \nu^k(A, B)$, and let $C_i^k = C_i \times \{k\}$. Then algorithm C1 describes how to draw from $Q_\nu(.|\nu)$.

Draw $C_i^k$ uniformly;
Draw $v$ a standard PRM;
$\nu' = g_{C_i^k}(\nu, v)$;

**Algorithm C1:** PRM proposal

## D. Implementation details

### *D.1. Simulation*

As already noted in the main text, the algorithm given in 1 is a simplification, as it considers that all the points of $\nu$ can be ordered by time, which is not the case, as $\nu$ has got an infinite number of points on any time interval. To simulate the process in finite time and memory, we need to be able to not look at the points of $\nu$ above some maximum rate.

If we had a upper bound on the event rates, we could just use that bound, and the algorithm 1 would be correct. In the absence of such a bound, we reuse our reformulation of the equation (2), and the division of $\mathbb{R}_+ \times \mathbb{R}_+$ into rectangles $A_{i,j}$.

For each event $k$, and each time column $i$, we will keep track of the index $j_{max}^{i,k}$ of the highest rectangle that we need to take into account. When we recompute the rates, we also update $j_{max}^{i,k}$ if the rate increases above the upper bound $u_{max}^{i,k}$. For each time column $i$, we also need to order all the points of the $(\nu^k)$ in the column up to the $(u_{max}^{i,k})$ by time, and we will write $(t_n^i, u_n^i, k_n^i)$ for this ordered set, where $k_n^i$ is the index of the event that the point belongs

**input :** The discrete measures $(\nu_k)_{k \leq K}$, the rates $(r_k)$, the increments $(\mu_k)$, and the initial condition $X_0 \in E$
**output:** Trajectory $(X_t)_{t \geq 0}$
Initialize $t_0 = 0$, $X_{t_0} = X_0$;
**for** $i = 1$ **to** $\infty$ **do**
    Determine $(j^{i,k}_{max})_k$, from $r_k(X_{t_i})$;
    Get the $N^i$ points of the $(\nu_k)$ below $u^k_{max}$, and order them by time $S^i = (t^i_n, u^i_n, k^i_n)_n$;
    Initialize $t^i_0 = t_i$ the left bound of $C_i$;
    **for** $n = 1$ **to** $N^i$ **do**
        **if** $u^i_n \leq r_{k^i_n}(X_{t^i_{n-1}})$ **then**
            $X_{t^i_n} = X_{t^i_{n-1}} + \mu_{k^i_n}$;
        **else**
            $X_{t^i_n} = X_{t^i_{n-1}}$;
        **end**
        Compute the new rates $r_k(X_{t^i_n})$;
        Update the remaining set of points to consider;
        **for** $k = 1$ **to** $K$ **do**
            **if** $r_k(X_{t^i_n}) > u^{i,k}_{max}$ **then**
                Increase $j^{i,k}_{max}$ as required, and update $S^i$;
            **end**
        **end**
    **end**
**end**

**Algorithm D2:** Exact simulation of a MJP from a PRM realisation

to. We can now write the more complex Algorithm D2, which remains exact as long as $j^{i,k}_{max}$ remains finite, that is as long as the solution does not explode.

A further refinement to Algorithm D2 that we use in practice is to also reduce $u^{i,k}_{max}$ when $r_k(X_{t_i})$ becomes low enough, $br_k(X_{t_i}) < u^{i,k}_{max}$.

Note further that to be consistent, when we draw points for a rectangle, everything should be as if those points had already been drawn. In particular, the points that we draw in one rectangle should not depend on what happens in some other column of $\nu$, because this would break independence. To ensure this, each column of $\nu$ uses its own pseudorandom number generator.

The approximate algorithm shortly described in the main text, that we use most often in practice, is given as algorithm D3.

**input :** The discrete measures $(\nu_k)_{k\leq K}$, the rates $(r_k)$, the increments $(\mu_k)$, and the initial condition $X_0 \in E$
**output:** Trajectory $(X_t)_{t\geq 0}$
Initialize $t_0 = 0$, $X_{t_0} = X_0$;
**for** $i = 1$ **to** $\infty$ **do**
  **for** $k = 1$ **to** $K$ **do**
    Determine the $r^i_k = r_k(X_{t_i})$;
    Determine $j^{i,k}_{max}$, from $r^i_k$;
    Count $N^i_k$ the points below $r^i_k$;
    $N^i_k = \sum_{j=1}^{j^{i,k}_{max}-1} \nu_k(A_{i,j}) + \sum_{n=1}^{\nu_k(A_{i,j^{i,k}_{max}})} \mathbb{1}_{u_n^{i,j,k} \leq r^i_k}$;
  **end**
  $X_{t_{i+1}} = X_{t_i} + \sum_{k=1}^{K} N^i_k \mu_k$;
**end**

**Algorithm D3:** Approximate simulation of a MJP from a PRM realisation

### *D.2. Source code*

The implementation is in the repository in
https://gitlab.com/bnguyenvanyen/ocamlecoevo/-/tree/master/sim/lib/ ,
in the files `prm.ml`, `ctmjp/ctmjp__Prm.ml`, and `ctmjp/ctmjp__Prm_approx.ml`.

## E. Additional details on the results

### *E.1. Methods comparison*

We provide here more details about the method comparison presented in section 4.1.

The target data is simulated with parameter values $\beta = 240\ year^{-1}$, $\nu = 80\ year^{-1}$, $\rho = 0.9$, $\frac{S_0}{N} = 0.9$, $\frac{I_0}{N} = 0.02$, $\frac{R_0}{N} = 0.08$, and with a population size $N$ taking values 500, 1000, 2000, 4000 and 8000.

Because of difficulties of implementation, the initial conditions priors are different between methods, and so we don't expect the results to be strictly identical.

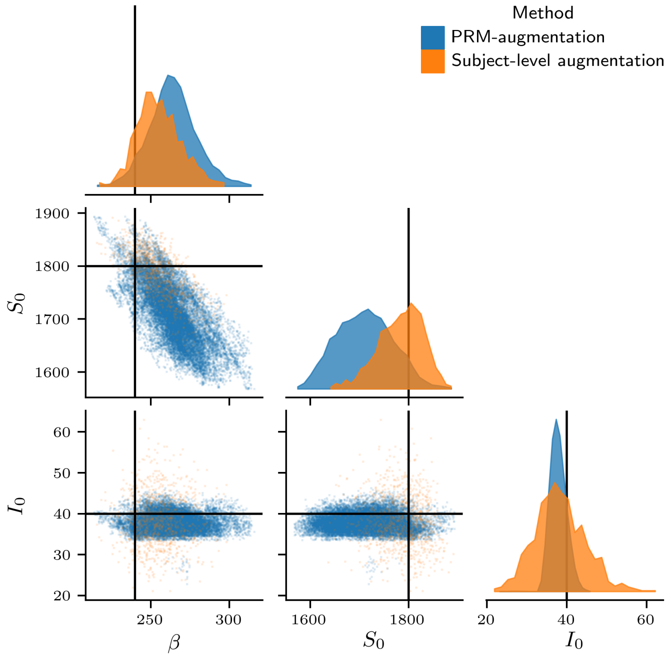


Figure E1: Parameter estimates for the simulated SIR data
In blue, results with PRM-augmented MCMC, and in orange, with subject-level augmentation.

The results of the estimation, for a population of 2000 hosts, are given in Fig. E1.

*E.2. Inference on simulated seasonal data*

In the results section 4.2, the data is simulated from a SEIRS model with vitality and seasonality.

The ODE for the model is given in equation (E.3), and the corresponding SDE in equation (E.4). $\nu^E$, $\nu^I$, $\nu^R$, $\nu^S$, $\nu^B$, $\nu^{SD}$, $\nu^{ED}$, $\nu^{ID}$, $\nu^{RD}$ are independent standard PRMs corresponding to the events of infection, becoming infectious, recovery, immunity loss, birth of a susceptible host, death of a susceptible host, death of an exposed host, death of an infectious host, and death of a removed host, respectively.

The parameter values are reproduced in Table E1 for completeness. The system is simulated for 10 years and the last 5 years of bi-weekly data are kept

for inference.

$$
\begin{aligned}
\frac{dS}{dt} &= -\beta(t)\frac{S}{N}(I+\eta) + \nu R + BN^* - DS \\
\frac{dE}{dt} &= \beta(t)\frac{S}{N}(I+\eta) - \sigma E - DE \\
\frac{dI}{dt} &= \sigma E - \gamma I - DI \\
\frac{dR}{dt} &= \gamma I - \nu R - DR \\
\frac{dC}{dt} &= \rho\beta(t)\frac{S}{N}(I+\eta) \\
N &= S + E + I + R \\
\beta(t) &= \beta_m + \beta_v sin(2\pi t + \phi)
\end{aligned}
\tag{E.3}
$$

$$
\begin{aligned}
S_t = S_0 + \int_0^t \int_{\mathbb{R}_+} & \big(\mathbb{1}_{u \le \nu R_{s^-}} \nu^S(ds,du) \\
& - \mathbb{1}_{u \le \lambda(s^-)} \nu^E(ds,du) \\
& + \mathbb{1}_{u \le BN^*} \nu^B(ds,du) \\
& - \mathbb{1}_{u \le DS_{s^-}} \nu^{SD}(ds,du)\ \big) \\
E_t = E_0 + \int_0^t \int_{\mathbb{R}_+} & \big(\mathbb{1}_{u \le \lambda(s^-)} \nu^E(ds,du) \\
& - \mathbb{1}_{u \le \sigma E_{s^-}} \nu^I(ds,du) \\
& - \mathbb{1}_{u \le DE_{s^-}} \nu^{ED}(ds,du)\ \big) \\
I_t = I_0 + \int_0^t \int_{\mathbb{R}_+} & \big(\mathbb{1}_{u \le \sigma E_{s^-}} \nu^I(ds,du) \\
& - \mathbb{1}_{u \le \gamma I_{s^-}} \nu^R(ds,du) \\
& - \mathbb{1}_{u \le DI_{s^-}} \nu^{ID}(ds,du)\ \big) \\
R_t = R_0 + \int_0^t \int_{\mathbb{R}_+} & \big(\mathbb{1}_{u \le \gamma I_{s^-}} \nu^R(ds,du) \\
& - \mathbb{1}_{u \le \nu R_{s^-}} \nu^S(ds,du) \\
& - \mathbb{1}_{u \le DR_{s^-}} \nu^{RD}(ds,du)\ \big) \\
C_t = \int_0^t \int_{\mathbb{R}_+} & \quad \mathbb{1}_{u \le \rho\lambda(s^-)} \nu^I(ds,du) \\
N_t = & \quad S_t + E_t + I_t + R_t \\
\beta(t) = & \quad \beta_m + \beta_v sin(2\pi t + \phi) \\
\lambda(t) = & \quad \beta(t)\frac{S(t)}{N(t)}(I(t)+\eta)
\end{aligned}
\tag{E.4}
$$

| | | |
|---|---|---|
| $B$ | Host birth rate | $\frac{1}{70}$ $years^{-1}$ |
| $D$ | Host death rate | $\frac{1}{70}$ $years^{-1}$ |
| $N^*$ | Base population size | 10000 |
| $\beta_m$ | Mean effective contact rate | 75 $years^{-1}$ |
| $\beta_v$ | Relative amplitude of effective contact rate | 0.4 |
| $\gamma$ | Recovery rate | 52 $years^{-1}$ |
| $\rho$ | Reporting probability | 0.5 |
| $\sigma$ | Becoming infectious rate | 26 $years^{-1}$ |
| $\nu$ | Immunity loss rate | 0.1 $years^{-1}$ |
| $\eta$ | Outside infectious population | 1 |
| $\phi$ | Contact rate phase | 0 |
| $dt$ | Sampling period | 0.01 $years$ |
| $t_f$ | Duration | 10 $years$ |
| $S_0$ | Initial population of susceptibles | 6250 |
| $E_0$ | Initial population of latent | 8 |
| $I_0$ | Initial population of infectious | 8 |
| $R_0$ | Initial population of resistant | 3734 |

Table E1: Parameter values for the simulated seasonal SEIRS dataset

Two versions of the model are used for inference. A seasonal version, where $\beta_v$ is fixed to its true value, and a constant version, where $\beta_v$ is fixed to 0.

The results of the parameter estimation are given in Fig. E2.

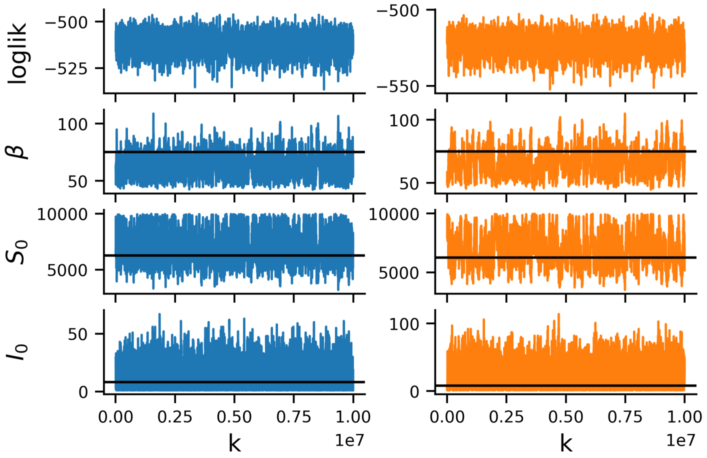


(a)

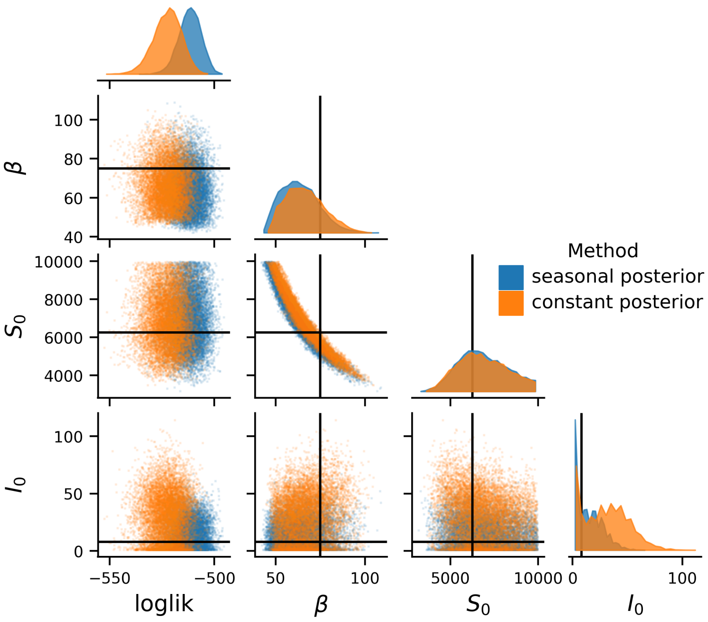


(b)

Figure E2: Parameter estimates for the simulated SEIRS seasonal data.
In blue, the prior distribution of the constant model. In orange, the posterior distribution of the seasonal model. In green, the posterior distribution of the constant model.
For the log-likelihood, and for the parameters $\beta$, $S_0$ and $I_0$. See Table E1 and Equation (E.3) for more details.
**(a)** MCMC traces for log-likelihood and parameters.
**(b)** MCMC samples pair scatter-plots for log-likelihood and parameters.

*E.3. Inference for Zika, French Polynesia, 2013-2014*

The model fit to the data is a SEIR model with immigration. It is the same as the previous SEIRS model (E.3), but without seasonality, host vitality, or immunity loss, which are not needed as the epidemic lasted only a few months.

We estimate the parameters $\beta$, $\sigma$, $\gamma$, and $\rho$. The prior distributions are in Table E2.

The results of the parameter estimation are shown in Fig. E3 for completeness, but as explained in the main text 4.3, the model does not describe the data well. Non-identifiability of the parameters and conflicts between the two sources of data hinders the mixing of the chain, and pushes the parameters $\beta$, $\sigma$ and $\gamma$ towards unrealistically high values. Indeed, without the upper bounds placed *a priori* on them, $\sigma$ and $\gamma$ reach values in the thousands, corresponding to incubation and infectious periods of a few hours.

| | | |
|---|---|---|
| $\beta$ | Effective contact rate | Lognormal $\mathcal{L}og(70, 0.1)$ |
| $\sigma$ | Becoming infectious rate | Uniform $\mathcal{U}([0, 100])$ |
| $\gamma$ | Recovery rate | Uniform $\mathcal{U}([0, 100])$ |
| $\rho$ | Reporting probability | Uniform $\mathcal{U}([0, 1])$ |
| $\eta$ | Outside infectious population | Fixed at 1 |
| $S_0$ | Initial population of susceptibles | Fixed at 17000 |
| $E_0$ | Initial population of exposed | Fixed at 0 |
| $I_0$ | Initial population of infectious | Fixed at 0 |
| $R_0$ | Initial population of removed | Fixed at 0 |

Table E2: Prior distributions for the Zika inference

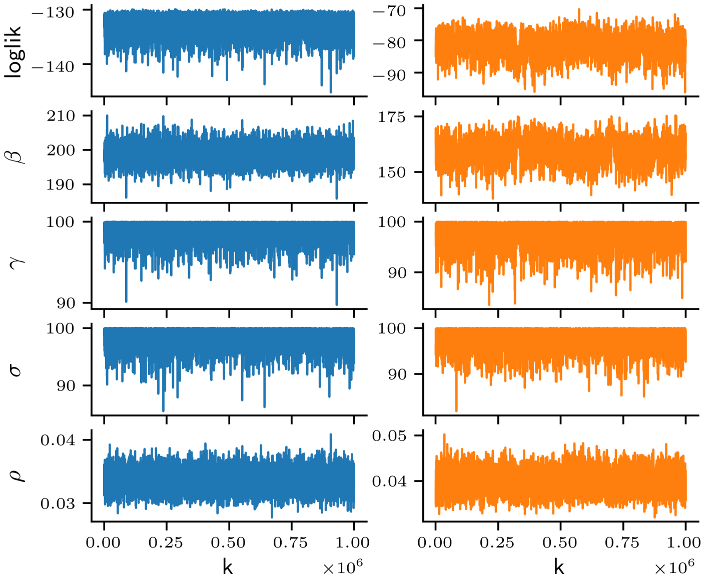


(a)

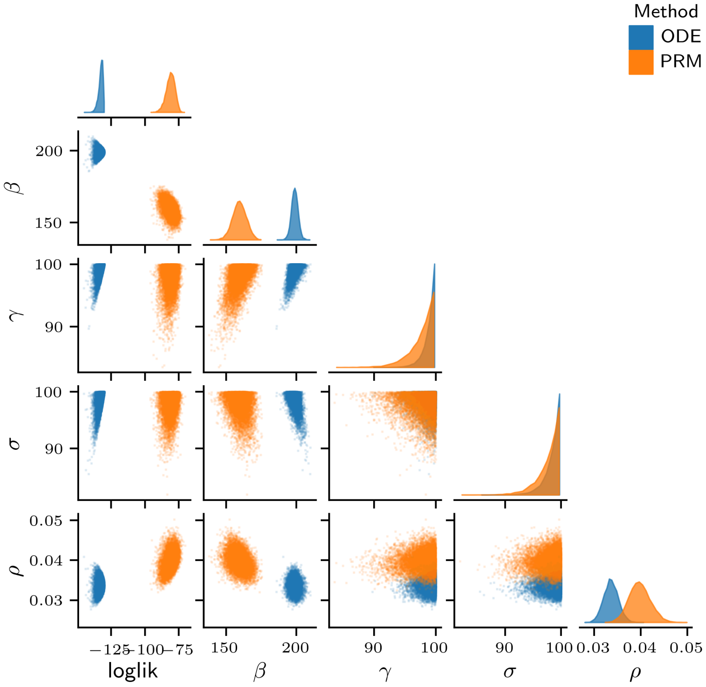


(b)

Figure E3: Parameter estimates for the French Polynesia Zika epidemic
In blue, the posterior distribution with the deterministic model. In orange, the posterior distribution with the stochastic model.
For the log-likelihood ("loglik"), and for the parameters $\beta$, $\gamma$, $\sigma$, and $\rho$. See Table E1 and Equation (E.3) for more details.
**(a)** MCMC traces for the log-likelihood and parameters.
**(b)** MCMC samples pair scatter-plots for the log-likelihood and parameters.

## F. Correctness and reproducibility

The repository at https://gitlab.com/bnguyenvanyen/ocamlecoevo contains 30000 lines of OCaml code relevant to the present paper. Our results rely on that code being bug-free. The choice of OCaml as programming language makes this easier than in C, C++, or python for example, thanks to the safety offered by type inference, as well as the use of immutability in most places, and the module system which enforces abstraction boundaries.

Mutability is still used in some performance-critical sections of the code, most notably the Poisson Random Measure implementation, at https://gitlab.com/bnguyenvanyen/ocamlecoevo/-/blob/master/sim/lib/prm.ml , so unit testing was also used.

It is difficult to test that the behaviour of random programs is correct, but we checked that the distribution of trajectories when simulating with PRM integration or with Gillespie's algorithm were very similar.

To facilitate reproducibility of the results, a repository with all the data, simulations, and MCMC outputs, as well as scripts to reproduce them, is at https://gitlab.com/bnguyenvanyen/article_prm_augmented_mcmc

The scripts to run the MCMC were adapted from the ones used in practice to run with Condor on the computing cluster at IBENS.

## References

[1] Jean Jacod and Albert N. Shiryaev. Characteristics of Semimartingales and Processes with Independent Increments. In *Limit theorems for stochastic processes*, number 288 in Grundlehren der mathematischen Wissenschaften. Springer, Berlin, 2. ed edition, 2010. OCLC: 846196420.

[2] Stewart N. Ethier and Thomas G. Kurtz. *Markov Processes: Characterization and Convergence*. John Wiley & Sons, September 2009.

[3] Nobuyuki Ikeda and Shinzo Watanabe. *Stochastic differential Equations and diffusion processes*. Number 24 in North-Holland mathematical Library. North-Holland [u.a.], Amsterdam, 2. ed edition, 1989. OCLC: 20080337.

[4] Mátyás Barczy, Zenghu Li, and Gyula Pap. Yamada-Watanabe Results for Stochastic Differential Equations with Jumps. *International Journal of Stochastic Analysis*, 2015.

[5] Fubao Xi and Chao Zhu. Jump type stochastic differential equations with non-Lipschitz coefficients: Non-confluence, Feller and strong Feller properties, and exponential ergodicity. *Journal of Differential Equations*, 266(8):4668–4711, April 2019.
